# Supplementary material for: An Economical Approach to Design with Precision Criteria
Source: arXiv:2306.09476 source file (2026-09-04)
Supplement: Supplementary file 1 [file length_supp.tex]

\documentclass{article}
\usepackage{color}
\usepackage{graphicx}
\usepackage{amsmath, amsthm}
\usepackage{mathtools}
\usepackage{natbib}
\usepackage{url}
\usepackage{soulutf8}
\RequirePackage[colorlinks,citecolor=blue,urlcolor=blue]{hyperref}
\usepackage{xcolor}
\usepackage{chngcntr}
\usepackage{subfig}
\usepackage{hyperref}
\usepackage{algorithm}
\usepackage[noend]{algpseudocode}
\usepackage{setspace}

\newtheorem{corollary}{Corollary}
\usepackage{xfrac}
\definecolor{forest}{rgb}{0.133,0.545,0.133}
\usepackage{multirow}
\usepackage{amsfonts}

\oddsidemargin=0in
\evensidemargin=\oddsidemargin
\textwidth=6.5in
\topmargin=-0.50in
\textheight=9.25in

\usepackage{etoolbox}

\newif\ifabbreviation
\pretocmd{\thebibliography}{\abbreviationfalse}{}{}
\AtBeginDocument{\abbreviationtrue}

\begin{document}
	\newcommand{\bb}{\boldsymbol{\beta}}

	\title{Supplementary Material for `An Economical Approach to Design with Precision Criteria'}

	%% Group authors per affiliation:
 \author{}

	% \author{Luke Hagar\footnote{Luke Hagar is the corresponding author and may be contacted at \url{lmhagar@uwaterloo.ca}.} \hspace{35pt} Nathaniel T. Stevens \bigskip \\ \textit{Department of Statistics \& Actuarial Science} \\ \textit{University of Waterloo, Waterloo, ON, Canada, N2L 3G1}}

	\date{}

	\maketitle

% 	\begin{abstract}

% Equivalence testing allows one to conclude that two characteristics are practically equivalent. We propose a framework for fast sample size determination with Bayesian equivalence tests facilitated via posterior probabilities. We assume that data are generated using statistical models with fixed parameters for the purposes of sample size determination. Our framework leverages an interval-based approach, which defines a distribution for the sample size to control the length of posterior highest density intervals (HDIs). We prove the normality of the limiting distribution for the sample size, and we consider the relationship between posterior HDI length and the statistical power of Bayesian equivalence tests. We introduce two novel approaches for estimating the distribution for the sample size, both of which are calibrated to align with targets for statistical power. Both approaches are much faster than traditional power calculations for Bayesian equivalence tests. Moreover, our method requires users to make fewer choices than traditional simulation-based methods for Bayesian sample size determination. It is therefore more accessible to users accustomed to frequentist methods.

% 		\bigskip

% 		\noindent \textbf{Keywords:}
% 		Bayesian power analysis; design and analysis of experiments; interval-based sample size determination; practical equivalence; the Bernstein-von Mises theorem; two-group comparisons
% 	\end{abstract}

	\maketitle

	%\pagebreak
	\baselineskip=19.5pt

	%%%%%%%%%%%%%%%%%%%%%%%%%%%%%%%%%%%%%%%%%%%%%%%%%%%%%%%%%%%%%%%%%%%%%%%%%%%%%%%%%%%%%%%%%%%%%%%%%%%%%

 	\appendix
\numberwithin{equation}{section}
\renewcommand{\theequation}{\thesection.\arabic{equation}}

\numberwithin{figure}{section}
\renewcommand{\thefigure}{\thesection.\arabic{figure}}

\numberwithin{table}{section}
\renewcommand{\thetable}{\thesection.\arabic{table}}

\renewcommand{\thecorollary}{\Alph{corollary}}
	%%%%%%%%%%%%%%%%%%%%%%%%%%%%%%%%%%%%%%%%%%%%%%%%%%%%%%%%%%%%%%%%%%%%%%%%%%%%%%%%%%

\section{Detailed Description of the Regularity Conditions}\label{sec:proof}
% 	%%%%%%%%%%%%%%%%%%%%%%%%%%%%%%%%%%%%%%%%%%%%%%%%%%%%%%%%%%%%%%%%%%%%%%%%%%%%%%%%%%%%%%%%%%%%%%%%%%%%%
% 	%%%%%%%%%%%%%%%%%%%%%%%%%%%%%%%%%%%%%%%%%%%%%%%%%%%%%%%%%%%%%%%%%%%%%%%%%%%%%%%%%%%%%%%%%%%%%%%%%%%%%

\subsection{Conditions for the Asymptotic Normality of the Maximum Likelihood Estimator}\label{sec:MLE}
% 	%%%%%%%%%%%%%%%%%%%%%%%%%%%%%%%%%%%%%%%%%%%%%%%%%%%%%%%%%%%%%%%%%%%%%%%%%%%%%%%%%%%%%%%%%%%%%%%%%%%%%

Theorem 1 from the main text requires that the model $f^+(\boldsymbol{w}; \boldsymbol{\eta}^+)$ satisfies the regularity conditions for the asymptotic normality of the maximum likelihood estimator (MLE). These conditions should hold true for all $\boldsymbol{\eta}^+_{r} \sim \Psi$. These conditions are described in Theorem 5.39 of \citet{vaart1998bvm}. To align with the notation from \citet{vaart1998bvm}, we state these conditions in the context of a family of probability distributions $\mathcal{P} = \{P_{\theta}: \theta \in \Omega \}$, where $\Omega$ is the parameter space. Note that we have modified (R0) to accommodate settings with and without clustered data. Condition (R3) requires that the MLE of $\theta$ is consistent as $n \rightarrow \infty$.

% For our purposes, the conditions in \citet{lehmann1998theory} must hold for the models with unknown parameters $\boldsymbol{\eta}_1$ and $\boldsymbol{\eta}_2$ and true values $\boldsymbol{\eta}^*_{1}$ and $\boldsymbol{\eta}^*_{2}$.  

\begin{itemize}
    \item [(R0)] The data at the ISU level are drawn independently and identically from a distribution $P_{\theta_0}$ for some fixed, nonrandom $\theta_0$.
    \vspace*{-2pt}
    \item [(R1)] The parametric statistical model from which the data are generated is differentiable in quadratic mean.  
    \vspace*{-18pt}
    \item [(R2)] There exists a sequence of uniformly consistent tests for testing $H_0: \theta = \theta_0$ against $H_1: \lVert \theta - \theta_0 \rVert \ge \varepsilon$ for every $\varepsilon > 0$.
    \vspace*{-2pt}
    \item [(R3)] The MLE $\hat{\theta}_n$ must be such that $\lvert \hat{\theta}_n - \theta_0 \rvert \overset{P}{\rightarrow} 0$ as $n \rightarrow \infty$.
\end{itemize}

	\subsection{Conditions for the Bernstein-von Mises Theorem}\label{sec:condBVM}
% 	%%%%%%%%%%%%%%%%%%%%%%%%%%%%%%%%%%%%%%%%%%%%%%%%%%%%%%%%%%%%%%%%%%%%%%%%%%%%%%%%%%%%%%%%%%%%%%%%%%%%%
% 	%%%%%%%%%%%%%%%%%%%%%%%%%%%%%%%%%%%%%%%%%%%%%%%%%%%%%%%%%%%%%%%%%%%%%%%%%%%%%%%%%%%%%%%%%%%%%%%%%%%%%

Theorem 1 from the main text also requires that the conditions for the Bernstein-von Mises (BvM) theorem are satisfied. These conditions are described in \citet{vaart1998bvm}, starting on page 140. Conditions (B0), (B1), and (B2) concern the likelihood component of the posterior distribution for a parameter $\theta$. These conditions are the same as conditions (R0), (R1), and (R2) for the BvM theorem that are listed in Appendix A.1. (B3) concerns the prior specifications for $\theta$. \citet{vaart1998bvm} uses $\theta_0$ instead of $\boldsymbol{\eta}_{r}$ as defined in Section 2 of the main text to refer to the fixed parameter value, so we again use that notation to state the conditions. The condition (B0) has been modified to accommodate settings with and without clustered data.

\begin{itemize}
    \item [(B0)] The data at the ISU level are drawn independently and identically from a distribution $P_{\theta_0}$ for some fixed, nonrandom $\theta_0$.
    \vspace*{-2pt}
    \item [(B1)] The parametric statistical model from which the data are generated is differentiable in quadratic mean.  
    \vspace*{-16pt}
    \item [(B2)] There exists a sequence of uniformly consistent tests for testing $H_0: \theta = \theta_0$ against $H_1: \lVert \theta - \theta_0 \rVert \ge \varepsilon$ for every $\varepsilon > 0$.
    \vspace*{-2pt}
    \item [(B3)] Let the prior distribution for $\theta$ be absolutely continuous in a neighbourhood of $\theta_0$ with continuous positive density at $\theta_0$.
\end{itemize}

	% 	%%%%%%%%%%%%%%%%%%%%%%%%%%%%%%%%%%%%%%%%%%%%%%%%%%%%%%%%%%%%%%%%%%%%%%%%%%%%%%%%%%%%%%%%%%%%%%%%%%%%%
% 	%%%%%%%%%%%%%%%%%%%%%%%%%%%%%%%%%%%%%%%%%%%%%%%%%%%%%%%%%%%%%%%%%%%%%%%%%%%%%%%%%%%%%%%%%%%%%%%%%%%%%

 \section{Proofs for Section 3}\label{sec:proof3}
	%%%%%%%%%%%%%%%%%%%%%%%%%%%%%%%%%%%%%%%%%%%%%%%%%%%%%%%%%%%%%%%%%%%%%%%%%%%%%%%%%%%%%%%%%%%%%%%%%%%%%
	%%%%%%%%%%%%%%%%%%%%%%%%%%%%%%%%%%%%%%%%%%%%%%%%%%%%%%%%%%%%%%%%%%%%%%%%%%%%%%%%%%%%%%%%%%%%%%%%%%%%%

     \subsection{Proof of Lemma 1}\label{sec:lem1}

     To prove Lemma 1 in the main text, we first consider the sampling distribution of the MLE for the model parameters $\boldsymbol{\eta}$ with respect to the number of ISUs $n$. We show that 
           \begin{equation}\label{eq:mle.param}
\sqrt{n}~ (\hat{\boldsymbol{\eta}}^{_{(n)}} - \boldsymbol{\eta}) \xrightarrow{d} N(\bf{0}, \bf{V}),
\end{equation} 
where $\bf{V}$ represents the information contribution in terms of an ``average" ISU as described below. In our framework, the ISU sizes are allowed to vary according to a given probability distribution. The size of a given ISU is encoded in the additional covariates ${\boldsymbol{X}}$, whose distribution is completely determined by the probability model $\Psi$.

The additional covariates -- regardless of whether they pertain to the ISU size -- impact the information about $\boldsymbol{\eta}$ contributed from a given ISU. We therefore define the expected information per ISU as 
           \begin{equation}\label{eq:exp.info}
\mathbb{E}_{{\boldsymbol{X}}} \left[ \mathcal{I}_{\text{ISU}}(\boldsymbol{\theta} \mid {\boldsymbol{x}}) \right] = {\bf{V}}^{-1},
\end{equation} 
where $ \mathcal{I}_{\text{ISU}}(\boldsymbol{\theta} \mid {\boldsymbol{x}})$ is the Fisher information according to the covariate pattern ${\boldsymbol{x}}$. The matrix ${\bf{V}}^{-1}$ in (\ref{eq:exp.info}) obtained by integrating over the selected probability distributions for ${\boldsymbol{X}}$ quantifies the information contribution from an average ISU. We assume the independent and identically distributed assumption holds at the ISU level and all remaining conditions for the asymptotic normality of the MLE are satisfied \citep{vaart1998bvm}. Thus, the limiting result in (\ref{eq:mle.param}) holds true in terms of the number of ISUs $n$.

The target of inference $\theta = g(\boldsymbol{\eta})$ in our framework is defined as a function of the model parameters $\boldsymbol{\eta}$. We obtain the sampling distribution of $\hat{\boldsymbol{\theta}}^{_{(n)}} = g(\hat{\boldsymbol{\eta}}^{_{(n)}})$ via the delta method:
           \begin{equation}\label{eq:mle.est}
\sqrt{n}~ \left(\hat{\boldsymbol{\theta}}^{_{(n)}} - g(\boldsymbol{\eta})\right) \xrightarrow{d} N\left(0, \frac{\partial g}{\partial \boldsymbol{\eta}}^{\emph{T}}{\bf{V}} \frac{\partial g}{\partial \boldsymbol{\eta}}\right).
\end{equation} 
Based on the result in (\ref{eq:exp.info}), the variance term in (\ref{eq:mle.est}) is $\lambda(\boldsymbol{\eta})$ as defined in Lemma 1. The approximate sampling distribution of $\hat{\boldsymbol{\theta}}^{_{(n)}}$ derived in Section 3 is therefore valid. In Section 3, we add the subscript $r$ to acknowledge that $\boldsymbol{\eta}_r \subseteq \boldsymbol{\eta}^+_r \sim \Psi$ may not be the same in all simulation repetitions. Since we assume the independent and identically distributed assumption holds at the ISU level and all remaining conditions for the BvM theorem are satisfied \citep{vaart1998bvm}, (\ref{eq:mle.est}) also guarantees the validity of our result in Lemma 1 of the main text. $\qed$

 \subsection{Proof of Theorem 1}\label{sec:thm1}

     We now prove Theorem 1 of the main text. The proof of Theorem 1 can be simplified by first verifying that the result in Corollary \ref{cora} holds true.

     \begin{corollary}\label{cora}
    Let $\mu_l =  4 z^2_{1-\alpha/2}\Lambda(\boldsymbol{\eta}_r)/l^2$ corresponding to a degenerate model $\Psi$, and let $V \in \{0,1\}$ denote whether the length criterion is satisfied. For large sample sizes $n$, $Pr(V = 1 |N = n)$ is approximately characterized by a univariate probit model with intercept $\beta_0 = -z_{1-\alpha/2}\Lambda(\boldsymbol{\eta}_r)^{\sfrac{1}{2}}/\mu_l^{\sfrac{1}{2}}$, slope $\beta_1 = z_{1-\alpha/2}\Lambda(\boldsymbol{\eta}_r)^{\sfrac{1}{2}}/\mu_l^{\sfrac{3}{2}}$, and error term variance $\sigma^2_{\varepsilon} = 4 z^2_{1-\alpha/2} \tau^2/\mu_l^{2}$.
\end{corollary}

        We first explain the rationale for how $\mu_l$ is defined. We define $\mu_l$ as the sample size $n$ such that the approximate normal distribution from (6) of the main text has mean of $l$. Equating the mean of this approximate distribution to $l$ and solving for $n$ yields
    \begin{equation}\label{eqn:sssd_mean}
    \mu_l = \dfrac{4 z^2_{1-\alpha/2}\Lambda(\boldsymbol{\eta}_r)}{l^2}.
    \end{equation}
    We note that $\mu_l \rightarrow \infty$ as $l \rightarrow 0^+$. We define a variable $V \in \{0, 1\}$ that denotes whether the length criterion is satisfied. That is, $V = 1$ if and only if $l - L_{1 - \alpha}(\boldsymbol{W}^{_{(n)}}) \ge 0$. By (6) of the main text, $l - L_{1 - \alpha}(\boldsymbol{W}^{_{(n)}})$ is approximately normal for a given large sample size $n$. We let $N$ be a random variable for the sample size. We now show that conditional on the sample size, the probit model given by
    	\begin{equation}\label{eqn:probit}
		\Phi^{-1}(Pr(V = 1 |N = n)) = \dfrac{-z_{1-\alpha/2}\Lambda(\boldsymbol{\eta}_r)^{\sfrac{1}{2}}}{\mu_l^{\sfrac{1}{2}}} + \dfrac{z_{1-\alpha/2}\Lambda(\boldsymbol{\eta}_r)^{\sfrac{1}{2}}}{\mu_l^{\sfrac{3}{2}}}n,
	\end{equation} 
where the model's error terms have homoscedastic variance $\sigma_{\varepsilon}^2 = 4 z^2_{1-\alpha/2} \tau^2/\mu_l^{2}$ approximately characterizes $Pr(V = 1 |N = n)$ for large sample sizes $n$. The function $\Phi(\cdot)$ denotes the standard normal cumulative distribution function (CDF).

The intercept $\beta_0$ and slope $\beta_1$ of the probit model in (\ref{eqn:probit}) define the first-order Taylor approximation to $l - \mathbb{E}(L_{1 - \alpha}(\boldsymbol{W}^{_{(n)}}))$ at $n = \mu_l$. For large sample sizes $n$ in a neighbourhood of $\mu_l$, $\beta_0 + \beta_1n \approx l - \mathbb{E}(L_{1 - \alpha}(\boldsymbol{W}^{_{(n)}}))$. It follows from (6) of the main text that the approximately normally distributed error terms for $l - L_{1 - \alpha}(\boldsymbol{W}^{_{(n)}})$ exhibit heteroscedasticity: $Var(L_{1 - \alpha}(\boldsymbol{W}^{_{(n)}})) \approx 4z_{1-\alpha/2}^2\tau^2/n^2$ decreases as $n$ increases. We demonstrate shortly that the impact of this heteroscedasticity is negligible for large $n$, and we can treat the error terms as having homoscedastic variance $\sigma_{\varepsilon}^2$. 

If the probit model from (\ref{eqn:probit}) is appropriate, then $N$ is normally distributed with mean $-\beta_0/\beta_1$ and standard deviation $\sigma_{\varepsilon}/\beta_1$. It follows by (\ref{eqn:probit}) that $-\beta_0/\beta_1 = \mu_l$. The standard deviation, which we denote $\sigma_{l, \mu_l}$, is given by
    	\begin{equation}\label{eqn:sigmal}
 \dfrac{\sigma_{\varepsilon}}{\beta_1} = \dfrac{2z_{1-\alpha/2}\tau/\mu_l}{z_{1-\alpha/2}\Lambda(\boldsymbol{\eta}_r)^{\sfrac{1}{2}}/\mu_l^{\sfrac{3}{2}}} = 4z_{1-\alpha/2}\tau/l,
	\end{equation} 
where the last equality is obtained by substituting the expression for $\mu_l$ from (\ref{eqn:sssd_mean}). 

% Theorem 1 states that the standard deviation of the SSSD $\sigma_l = \sigma/l$ involves a constant $\sigma$.

The value for $l \sigma_{l, \mu_l} = 4z_{1-\alpha/2}\tau$ was obtained using $\sigma^2_{\varepsilon} = Var(L_{1 - \alpha}(\boldsymbol{W}^{_{(\mu_l)}}))$. For given $l$, we obtain a different value for this quantity using the approximate distribution of $L_{1 - \alpha}(\boldsymbol{W}^{_{(n)}})$ for $n \ne \mu_l$. We call this quantity $l \sigma_{l,n}$ and consider $n = \mu_l + a$ for $\lvert a \rvert < c\sigma_{l, \mu_l}$ for some sufficiently large constant $c > 0$. To show that the impact of heteroscedasticity is negligible for large sample sizes $n$, we consider the limiting behaviour of $l \sigma_{l,n}$. By substituting the square root of (\ref{eqn:sssd_mean}) for $\mu_l^{\sfrac{1}{2}}$ in the second line of the following equation, we obtain a simplified expression for $l \sigma_{l,n}$:
\begin{align}
 l\sigma_{l,n} &=\dfrac{l \times Var(L_{1 - \alpha}(\boldsymbol{W}^{_{(n)}}))}{\beta_1} \nonumber \\
 &=\dfrac{l \times 2z_{1-\alpha/2}\tau/n}{\dfrac{z_{1-\alpha/2}\Lambda(\boldsymbol{\eta}_r)^{\sfrac{1}{2}}}{\mu_l^{\sfrac{1}{2}}} \div \mu_l} \nonumber \\
&= 4z_{1-\alpha/2}\tau \times \dfrac{\mu_l}{n} \nonumber
\\ &= 4z_{1-\alpha/2}\tau \times \dfrac{1}{1 + a/\mu_l}. \label{eqn:hetero}
\end{align}
The limit of (\ref{eqn:hetero}) is $4z_{1-\alpha/2}\tau$ as $l \rightarrow 0^+$ since $\mu_l$ and $\lvert a \rvert \propto \sigma_l$ are functions of $l^{-2}$ and $l^{-1}$, respectively. It follows that for arbitrary fixed $a$, $\lim_{\mu_l \rightarrow \infty}l\sigma_{l, \mu_l + a}$ $= 4z_{1-\alpha/2}\tau = l\sigma_{l, \mu_l}$. For large sample sizes $n = \mu_l + a$, $l\sigma_{l,n}$ does not change drastically, so the impact of heteroscedasticity is not substantial. Therefore, Corollary \ref{cora} holds true: the probit model from (\ref{eqn:probit}) approximately characterizes $Pr(V = 1 |N = n)$ for large sample sizes $n$. $\qed$

 Lastly, we use Corollary \ref{cora} to prove Theorem 1 of the main text. We let $\sigma_l = \sigma_{l, \mu_l} = 4z_{1-\alpha/2}\tau/l$. In (\ref{eqn:hetero}), we considered sample sizes in the interval $\{ n ~|~ n \in (\mu_l ~\pm~ c\sigma_l)\}$. As $l \rightarrow 0^+$, both the lower and upper extremes of this interval approach $\infty$ because $\mu_l$ and $\sigma_l$ are respectively functions of $l^{-2}$ and $l^{-1}$. Because the probit model from Corollary \ref{cora} is appropriate for the sample sizes in this interval, it follows that
     	\begin{equation}\label{eqn:ks1}
\lim_{l\rightarrow 0^+}	\sup_{n \in \mathbb{Z}^+: n \in (\mu_l ~\pm~ c\sigma_l)} \left\lvert F_l(n) - \Phi\left(\dfrac{n - \mu_l}{\sigma_l}\right) \right\rvert \xrightarrow{P} 0.
	\end{equation} 
 We note that the discreteness of the sample size $n$ does not impact the quality of the normal approximation for large sample sizes $n$, where $\sigma_l$ is also large. The result in (\ref{eqn:ks1}) also holds true for $n \in \mathbb{Z}^+: n \le \mu_l - c\sigma_l$ in the limiting case. As $l \rightarrow 0^+$, both $F_l(n)$ and $\Phi\left((n - \mu_l)/\sigma_l\right)$ converge in probability to 0. The result in (\ref{eqn:ks1}) additionally holds true for $n \in \mathbb{Z}^+: n \ge \mu_l + c\sigma_l$ in the limiting case. As $l \rightarrow 0^+$, both $F_l(n)$ and $\Phi\left((n - \mu_l)/\sigma_l\right)$ converge in probability to 1. The result in (\ref{eqn:ks1}) therefore extends to all $n \in \mathbb{Z}^+$, which formally proves Theorem 1 of the main text.  $\qed$

 \section{Additional Numerical Studies}

 In this appendix, we use several straightforward examples to further assess the performance of our approaches to estimate the LP distribution. While analytical estimation of the LP distribution is accurate when the underlying normal approximations are suitable, the following numerical studies illustrate that Algorithm 2 yields good performance more generally. The examples we consider concern a single group of independently and identically distributed normal data $\{y_i\}_{i=1}^n \sim \mathcal{N}(\mu, \sigma^2)$. We first estimate the LP distribution in a context where a 95\% CI for $\theta = \mu$ should have length at most $l = 0.6$. We can suppose that we want the length criterion to be satisfied with probability of at least $q = 0.8$. However, we focus more on the quality of LP curve approximation than the resulting sample size recommendations in this appendix. 

    We first consider the conditional approach. In this case, we suppose that observations are generated from the $\mathcal{N}(\mu_r = 5,\sigma^2_r = 2)$ distribution across simulation repetitions $r = 1, \dots, m$. The parameters $\mu_r$ and $\sigma^2_r$ are separate from the parameters of the normal approximation to the LP distribution: $\mu_l$ and $\sigma_l$. For this simple model, we can easily find the analytical approximation to the LP distribution from Theorem 1. We have that $\boldsymbol{\eta} = (\mu, \sigma^2)$ and $g(\boldsymbol{\eta}_r) = \mu_r$. It follows that $$\Lambda(\boldsymbol{\eta}_r) = \begin{pmatrix}
        1 \\ 0
    \end{pmatrix}^{\text{T}} \begin{bmatrix}
        \sigma_r^2 & 0 \\ 0 & 2\sigma_r^4 
    \end{bmatrix}\begin{pmatrix}
        1 \\ 0
    \end{pmatrix} = \sigma_r^2.$$
    Thus, $\mu_l =  4 z^2_{1-\alpha/2}\sigma_r^2/l^2$ since $\Lambda(\boldsymbol{\eta}_r) = \sigma_r^2$. By the delta method, $\tau = \sigma^2_r/2$ and  $\sigma_l = 2\sqrt{2}z_{1-\alpha/2} \sigma_r/l$. For this $\mathcal{N}(\mu_r = 5,\sigma^2_r = 2)$ example, $\mu_l = 85.37$ and $\sigma_l = 13.07$. 

    We consider several methods to construct 95\% CIs for $\mu$. In a Bayesian setting, we use a conjugate normal-gamma prior for $(\mu, \sigma^{-2})$. The marginal posterior for $\mu$ therefore follows a location-scale $t$-distribution. We consider three such prior distributions. First, $\text{NG}(\mu = 0,\lambda = 1,\alpha = 2,\beta = 2)$ serves as a diffuse prior. Second,  $\text{NG}(\mu = 0,\lambda = 10,\alpha = 2,\beta = 2)$ serves as a misspecified prior since the value of $\mu_r$ is 5 and $\lambda = 10$ is non-negligible. Third, $\text{NG}(\mu = 5,\lambda = 10,\alpha = 2,\beta = 2)$ serves as a correctly specified prior. We also consider the standard frequentist method to construct 95\% CIs based on the Student's $t$-distribution. In Figure \ref{fig:cond}, we consider these four scenarios. For each scenario, we approximate the LP curve using Algorithm 2 with only two estimates of the sampling distribution of CI lengths, each with $m = 10^4$ simulation repetitions. We also approximate the LP curve using naive simulation to estimate the sampling distribution of CI lengths in increments of $n = 5$ across the $x$-axis. We plot the analytical approximation to the LP curve provided above in each subplot; this analytical curve is the same for all four scenarios since Theorem 1 is based solely on large-sample theory. 

        \begin{figure}[!tb]
		\includegraphics[width = \textwidth]{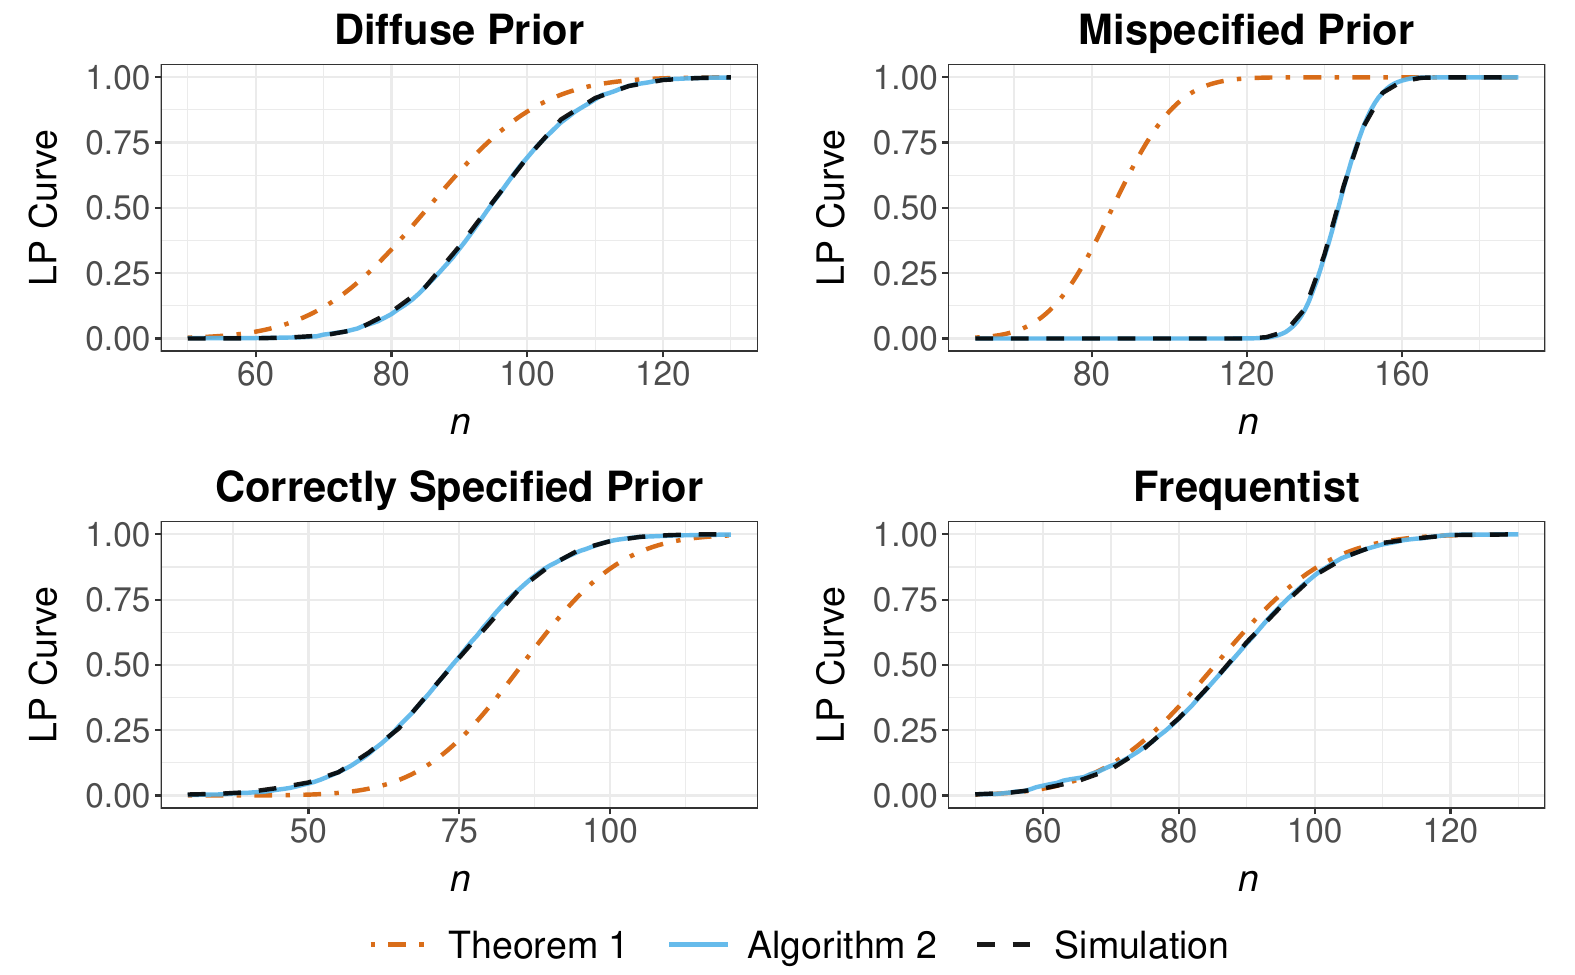} 

		\caption{\label{fig:cond} LP curves obtained using various estimation methods when the mean is the target of inference under the conditional approach. } 
	\end{figure}

    Even with the moderate sample sizes for this example, Algorithm 2 performs very well when approximating the LP curve compared to naive simulation since the solid and dashed curves essentially overlap. However, the analytical approximation to the LP curve from Theorem 1 is less accurate. In the frequentist case, the dot-dash curve is shifted slightly to the left because the empirical CI lengths are based on a $t$-distribution, whereas Theorem 1 leverages asymptotically normal sampling distributions. That is, the empirical CI lengths are a bit longer. The discrepancy between the $t$-distribution and normal distribution also impacts the Bayesian plots. Moreover, we generally require less (more) data if the prior is (mis)specified. The subpar performance of the analytical approximation to the LP curve for the Bayesian implementations of this example underscores the need for efficient simulation-based methods like Algorithm 2. 

    Once again, Theorem 1 provides an instantaneous normal approximation to the LP distribution. Roughly 20 seconds on a high-computing server with 72 cores were required approximate the LP curve via Algorithm 2 for each subplot in Figure \ref{fig:cond}. It took approximately 3 minutes using the same computing resources to approximate these LP curves using naive simulation when simulating sampling distributions of CI lengths in increments of $n = 5$. Alternatively, one could obtain a suitable sample size recommendation (but not approximate the entire LP curve) by exploring the sample size space via binary search. For the settings in Figure \ref{fig:cond}, it takes roughly 80 seconds to explore the $n$-space with binary search. The runtime discrepancy between using binary search and Algorithm 2 increases with the magnitude of the recommended $n$; regardless of the sample size recommendation, Algorithm 2 only requires that we estimate the sampling distribution of CI lengths at 2 values of $n$. The runtimes for the various methods described in this paragraph are similar for the following analyses in this appendix.

    We next consider the same 95\% CI construction methods (and prior distributions where applicable) under the predictive approach. For illustration, we now suppose the model $\Psi$ is such that $\sigma_r \sim \mathcal{U}[1, 1 + 2(\sqrt{2} - 1)]$. This uniform design prior for $\sigma_r$ is centered at the previous conditional value of $\sqrt{2}$. We let $\mu_r = 5$ for $r = 1, \dots, m$ because, as demonstrated above, the normal approximation to the LP curve does not depend on $\mu_r$ for this example. The analytical approximation to the LP distribution is a mixture of normal distributions that we obtain by applying Theorem 1 to 1000 simulated $\sigma_r$ values.      Figure \ref{fig:pred} provides LP curve visualizations for the predictive approach that are similar to those in Figure \ref{fig:cond}. Again, the LP distributions under the predictive approach exhibit greater dispersion than those under the conditional approach. For the Bayesian settings, Algorithm 2 better aligns with the results from naive simulation. To accommodate the predictive approach with Algorithm 2, the CI lengths were split into 10 bins based on the true $\sigma_r$ value at each sample size before constructing the linear approximations. 

            \begin{figure}[!tb]
		\includegraphics[width = \textwidth]{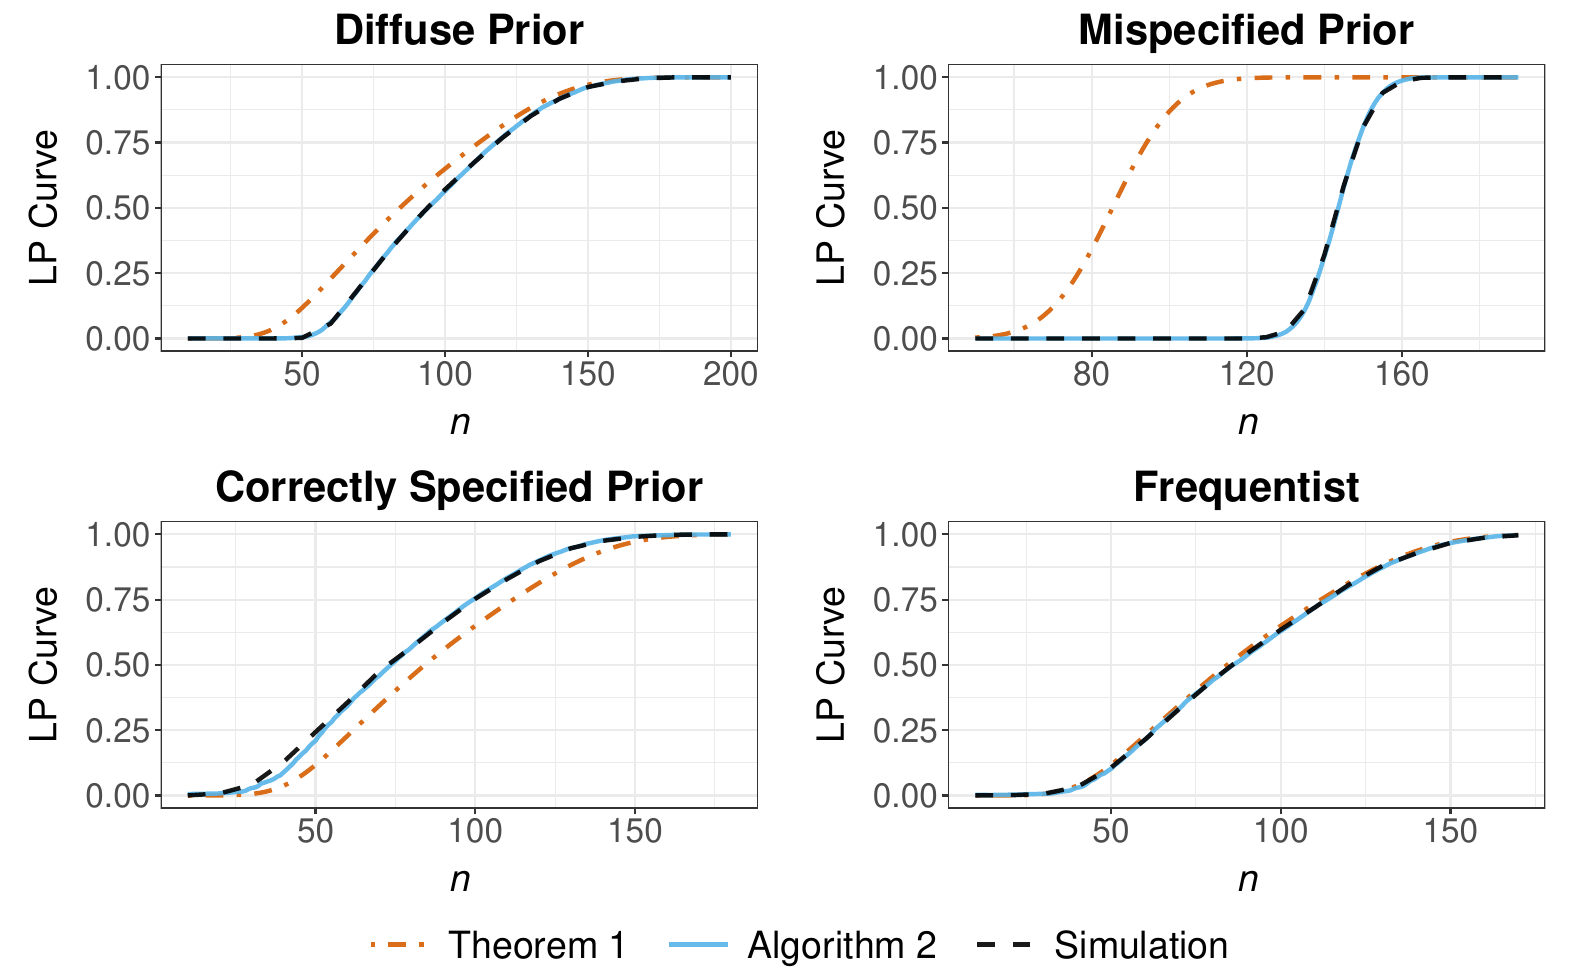} 

		\caption{\label{fig:pred} LP curves obtained using various estimation methods when the mean is the target of inference under the predictive approach.} 
	\end{figure}

    \begin{figure}[!tb]
		\includegraphics[width = \textwidth]{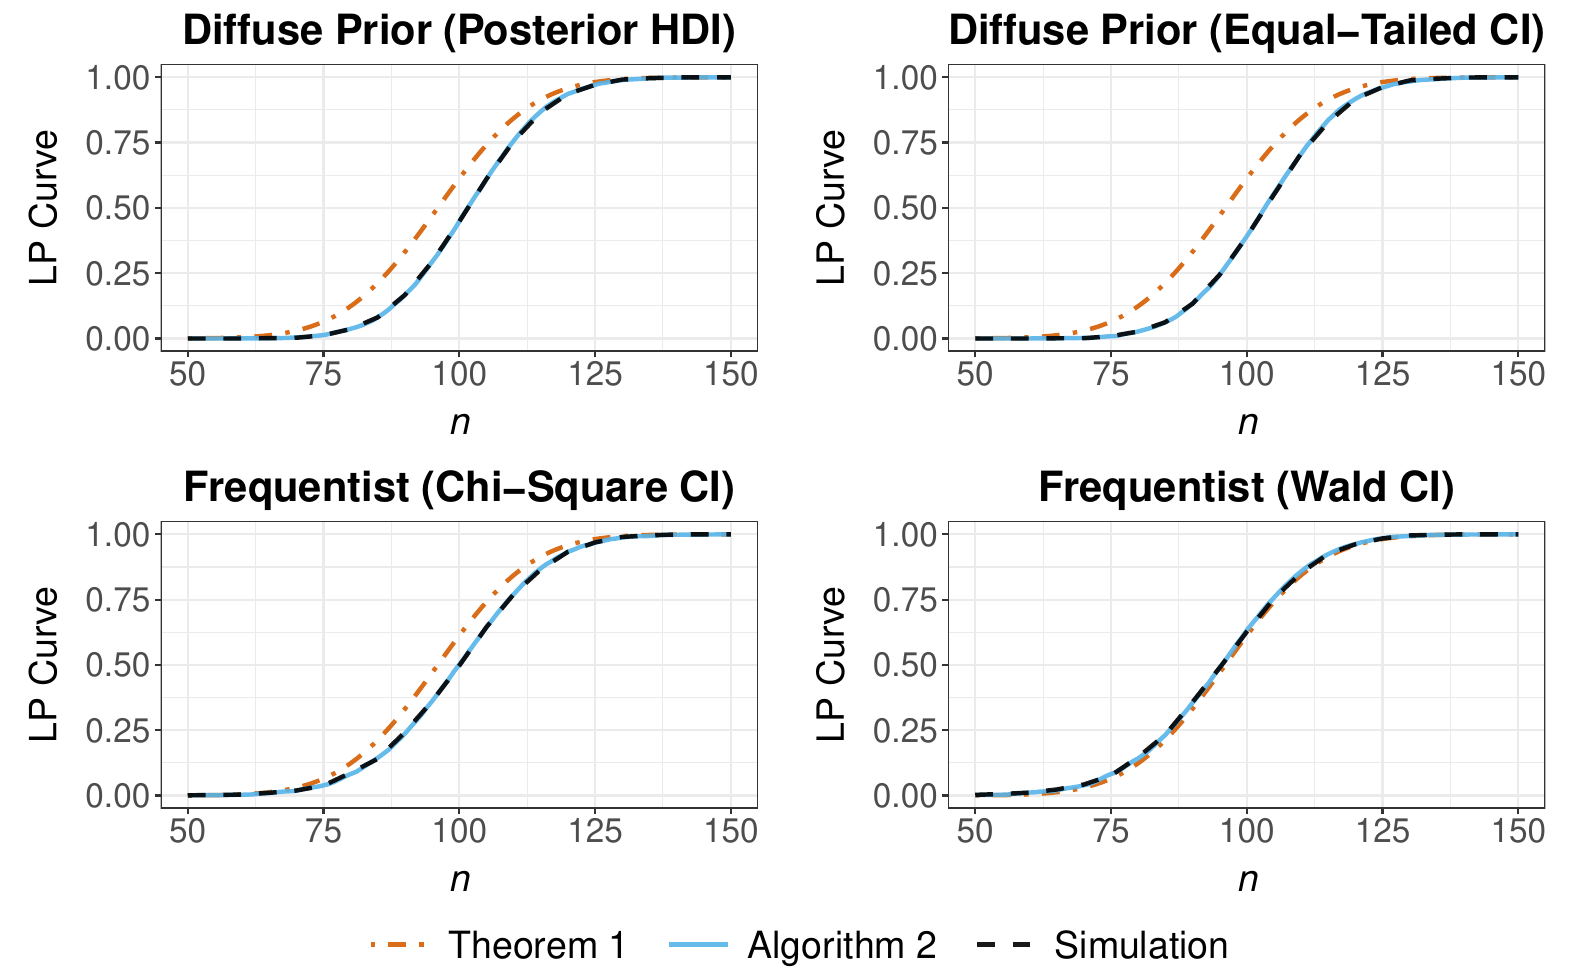} 

		\caption{\label{fig:sd} LP curves obtained using various estimation methods when the standard deviation is the target of inference. } 
	\end{figure}

    Lastly, we explore the performance of our methods to approximate the LP curve when the underlying posterior distributions or test-statistic sampling distributions are skewed. For this purpose, we reconsider the conditional approach where all observations are generated from the $\mathcal{N}(\mu_r = 5,\sigma^2_r = 2)$ distribution for $r = 1, \dots, m$. We now consider the length of the 95\% CI for the standard deviation (i.e., $\theta = \sigma$). Using Theorem 1, the parameters of the normal approximation to the LP curve are $\mu_l =  2 z^2_{1-\alpha/2}\sigma_r^2/l^2$ and  $\sigma_l = 2z_{1-\alpha/2} \sigma_r/l$. For this $\mathcal{N}(\mu_r = 5,\sigma^2_r = 2)$ example with $l = 0.4$, $\mu_l = 96.04$ and $\sigma_l = 13.86$. In the Bayesian paradigm, we only consider the diffuse prior from the earlier plots. However, we now consider two methods to construct the 95\% CI: the posterior highest density interval (HDI) and an equal-tailed CI. For the frequentist setting, we construct a 95\% CI for $\sigma$ by first constructing a 95\% CI for $\sigma^2$ based on exact pivotal quantities from the chi-square distribution and transforming the interval endpoints. We also construct an approximate 95\% Wald-based CI. Figure \ref{fig:sd} provides visualizations of the approximated LP curves when $\theta = \sigma$.

         The analytical approximation to the LP curve performs well when using frequentist Wald-based CIs, which makes sense because the large-sample theory is tailored to this case. However, the analytical approximation to the LP curve underestimates the required sample size in all other settings. This underestimation occurs because the underlying true posterior distribution (or chi-square distribution of the test statistic) has a right tail that increases the value of the upper CI endpoint. Nevertheless, Algorithm 2 can accommodate asymmetric CIs, and it performs very well at approximating the LP curve in comparison to naive simulation. Thus, efficient simulation-based methods for design with precision criteria are important when asymmetric CIs are constructed.

\bibliographystyle{chicago}
% \bibliography{length_supp}

\end{document}
